# Supplementary material for: Predicting Unconventional High Temperature Superconductors in Trigonal Bipyramidal Coordinations
Source: arXiv:1506.03904 source file (2015-06-19)
Supplement: Supplementary file 1 [file supplementary-r2.pdf]

# Supplementary materials

(Dated: June 19, 2015)

PACS numbers: 74.70.-b, 74.25.Ha, 74.20.Pq

In this supplementary, we investigate the electronic structures of possible materials constructed by the trigonal bipyramidal complexes under $3d^7$ filling configurations. Our density functional theory calculations employ the projector augmented wave (PAW) method encoded in Vienna ab initio simulation package(VASP)[1–3], and the generalized-gradient approximation (GGA) for the exchange correlation functional is used[4]. The cutoff energy of 500 eV is taken for expanding the wave functions into plane-wave basis. In the calculation, the number of these k points is ($16 \times 16 \times 6$) for the nonmagnetic calculations and ($9 \times 9 \times 5$) for the magnetic calculations. The GGA plus on-site repulsion U method (GGA+U) in the formulation of Dudarev *et al.*[5] is employed to describe the electron correlation effect associated with the Ni/Co $3d$ states by an effective parameter $U_{eff}$. The value of $U_{eff} = 4eV$ on Ni/Co is adopted in the calculations. The lattice constants and internal atomic positions are fully relaxed.

Fig.1 shows the crystal structure of $AMOX_2$ (A=Y,K,Ba,Yb, M=Ni,Co,Pd and X=F,Cl,O). The transition metal ions are surrounded by trigonal bipyramidal arrangements of anions. The band structure of $YNiO_3$ has been given in the main text. The Fermi surfaces are mainly contributed by $d_{xy}$ and $d_{x^2-y^2}$ orbitals of Ni. To investigate the magnetic properties we perform the GGA+U calculations for different magnetic states. The in-out AFM magnetic state in the triangle lattice is found to have a large energy gain about 0.35 eV per Ni relative to the paramagnetic state. From this energy, we estimate that the nearest neighbor AFM exchange couplings are about $0.1ev$ which is close to the values in cuprates. The band structure of $YNiO_3$ with the in-out AFM state is shown in Fig.2. We find that the system becomes a Mott insulator with a gap of 0.024 eV in the AFM state.

Like the multi-layer cuprates, we also consider a possible two-layer NiO material $YbNi_2O_4$, where the trigonal bipyramids in the two layers are connected by sharing edges. The crystal structure and band structure are given in Fig.3. In contrast to $YNiO_3$, $d_{yz}$ and $d_{xz}$ also contribute to the Fermi surfaces in $YbNi_2O_4$ due to the strong coupling between the two NiO layers. This result suggests that this multi-layer structure likely will not enhance $T_c$, in contrast to cuprates.

We also consider other possible Ni, Co and Pd based materials with the trigonal bipyramidal crystal field, whose band structures are shown in Fig.4. We find that the states near the Fermi level are mainly attributed to $d_{xy}$ and $d_{x^2-y^2}$ orbitals in all materials. For the Ni based materials, the effective hopping though the anions between the nearest-neighbor Ni is large, making the $d_{xy}$ and $d_{x^2-y^2}$ bands dispersive. For the Pd based materials, the $d_{xy}$ and $d_{x^2-y^2}$ bandwidth is larger due to the extended $4d$ orbitals. However, the effective hopping in Co-based materials is much smaller. These results suggest that there are rich classes of materials to explore the correlated electron physics.

In summary, there are many possible materials that can provide the desired electronic structure proposed in the main text. One can also replace elements in these materials by other elements with an identical valance to search stable crystal structures. High temperature superconductivity should be induced by doping these materials.

[1] G. Kresse and J. Hafner, Phys. Rev. B **47**, 558 (1993).
[2] G. Kresse and J. Furthmuller, Comput. Mater. Sci. **6**, 15 (1996).
[3] G. Kresse and J. Furthmuller, Phys. Rev. B **54**, 11169 (1996).
[4] J. P. Perdew, K. Burke, and M. Ernzerhof, Phys. Rev. Lett. **77**, 3865 (1996).
[5] S. L. Dudarev, G. A. Botton, S. Y. Savrasov, C. J. Humphreys, and A. P. Sutton, Phys. Rev. B **57**, 1505 (1998).

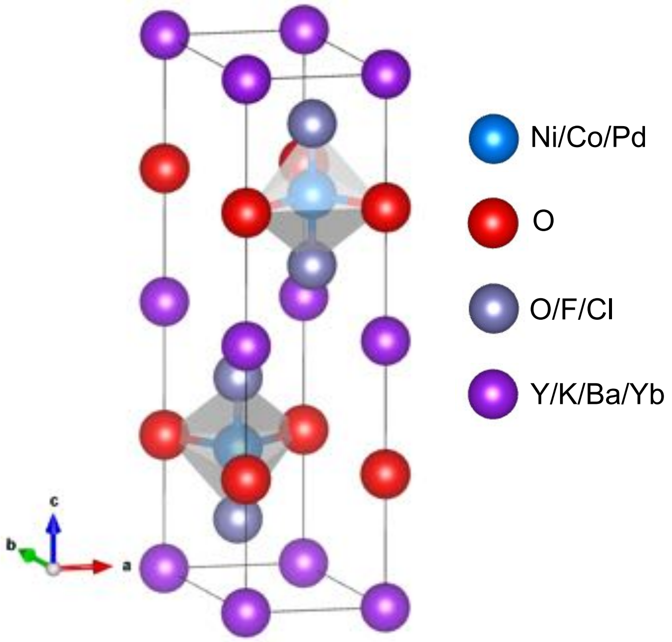


FIG. 1: The crystal structure of $AMOX_2$ (A=Y,K,Ba,Yb, M=Ni,Co,Pd and X=Cl,O).

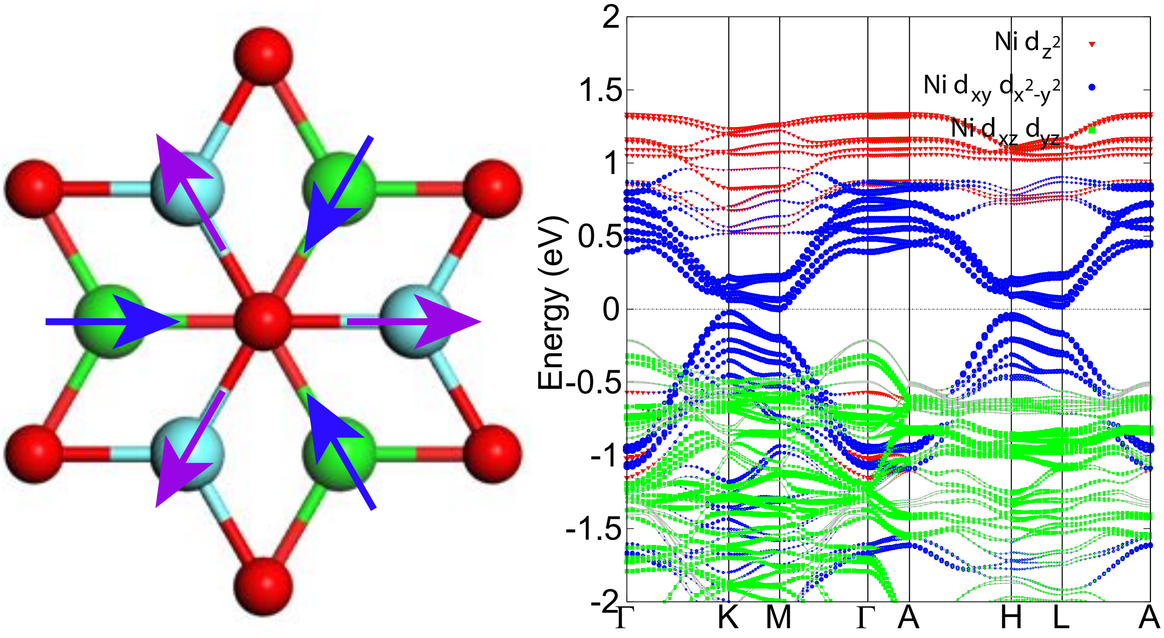


FIG. 2: The in-out AFM state and the GGA+U band structure of this state for $YNiO_3$.

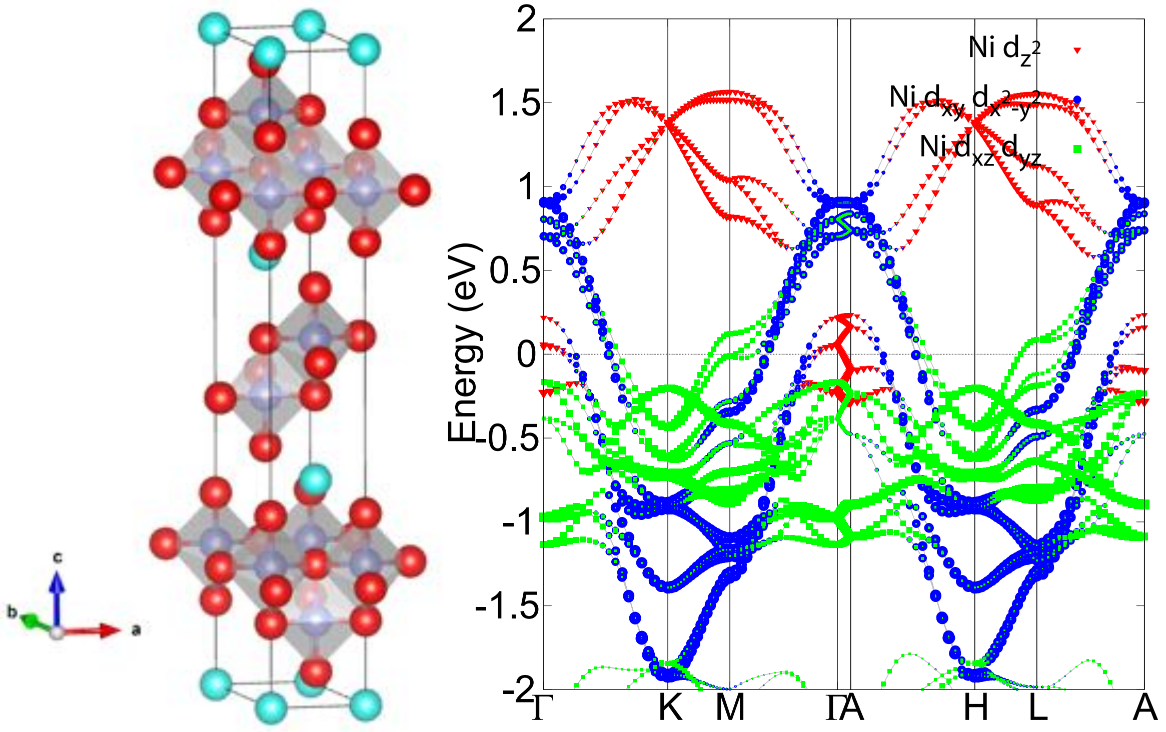


FIG. 3: The crystal structure and band structure of $YbNi_2O_4$.

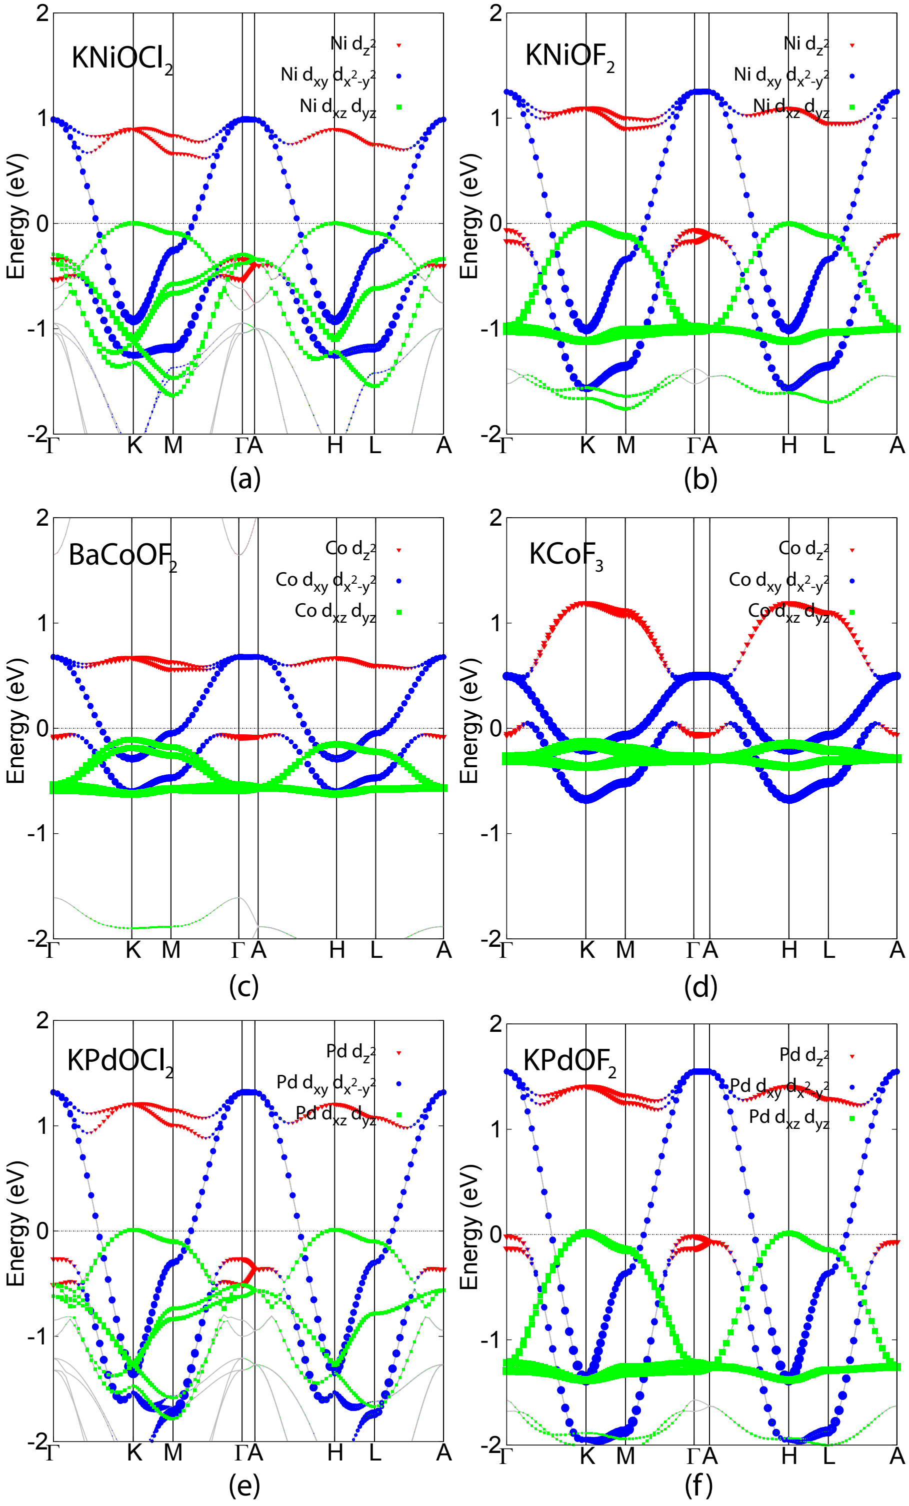


FIG. 4: The band structures of $KNiOCl_2$ (a), $KNiOF_2$ (b), $BaCoOF_2$ (c), $KCoF_3$ (d) $KPdOCl_2$ (e) and $KPdOF_2$ (f).
